# Supplementary material for: Toward Jordan Decompositions of Tensors
Source: arXiv:2206.13662 ancillary file (2024-07-08)
Supplement: Supplementary file 1 [file rank_profiles_trivectors.pdf]

# ADJOINT RANK PROFILES OF ALL ORBITS IN VINBERG AND ĖLAŠVILI'S CLASSIFICATION FOR $\wedge^3 \mathbb{C}^9$ .

FRÉDÉRIC HOLWECK AND LUKE OEDING

ABSTRACT. We provide the trace power invariants for general semisimple elements and the adjoint rank profiles of all orbits in Vinberg and Ėlašvili's classification for  $\wedge^3 \mathbb{C}^9$ , [?Vinberg-Elasvili] as an ancillary file to our article “Jordan Decompositions of Tensors.”

The orbits of  $SL_9$  in  $\wedge^3 \mathbb{C}^9$  occur in 7 families depending on the form of their semi-simple parts. Recall the basic semi-simple elements:

$$p_1 = e_0 e_1 e_2 + e_3 e_4 e_5 + e_6 e_7 e_8, \quad p_2 = e_0 e_3 e_6 + e_1 e_4 e_7 + e_2 e_5 e_8$$

$$p_3 = e_1 e_5 e_6 + e_2 e_3 e_7 + e_0 e_4 e_8, \quad p_4 = e_2 e_4 e_6 + e_0 e_5 e_7 + e_1 e_3 e_8$$

Here is the adjoint rank profile for random elements of each of the different families of semi-simple elements: We note that each of these families have non-zero values for their trace powers in degrees 12, 18, 24, 30, etc.

0.1. **Family one.** Basic semisimple form  $\sum_{i=1}^4 \lambda_i p_i$ . Block Ranks:  $\begin{pmatrix} 0 & 0 & 80 & 80 & 0 & 0 & 0 & 80 & 0 & 240 \\ 0 & 80 & 0 & 0 & 0 & 80 & 80 & 0 & 0 & 240 \end{pmatrix}$

The trace powers on generic semi-simple elements are:

$$f_{12} = (\lambda_1^{12} + 22 \lambda_1^6 \lambda_2^6 + \lambda_2^{12} - 220 \lambda_1^6 \lambda_2^3 \lambda_3^3 - 220 \lambda_1^3 \lambda_2^6 \lambda_3^3 + 22 \lambda_1^6 \lambda_3^6 + 220 \lambda_1^3 \lambda_2^3 \lambda_3^6 + 22 \lambda_2^6 \lambda_3^6 + \lambda_3^{12} - 220 \lambda_1^6 \lambda_2^3 \lambda_3^3 + 220 \lambda_1^3 \lambda_2^6 \lambda_3^3 - 220 \lambda_1^6 \lambda_3^3 \lambda_4^3 + 220 \lambda_2^6 \lambda_3^3 \lambda_4^3 - 220 \lambda_1^3 \lambda_2^3 \lambda_4^3 + 220 \lambda_2^6 \lambda_3^3 \lambda_4^3 + 22 \lambda_1^6 \lambda_2^6 - 220 \lambda_1^3 \lambda_2^3 \lambda_4^6 + 22 \lambda_2^6 \lambda_4^6 + 220 \lambda_1^3 \lambda_3^3 \lambda_4^6 + 220 \lambda_2^3 \lambda_3^3 \lambda_4^6 + 22 \lambda_3^6 \lambda_4^6 + \lambda_4^{12}) (4536)$$

$$f_{18} = (\lambda_1^{18} - 17 \lambda_1^{12} \lambda_2^6 - 17 \lambda_1^6 \lambda_2^{12} + \lambda_2^{18} + 170 \lambda_1^{12} \lambda_2^3 \lambda_3^3 + 1870 \lambda_1^9 \lambda_2^6 \lambda_3^3 + 1870 \lambda_1^6 \lambda_2^9 \lambda_3^3 + 170 \lambda_1^3 \lambda_2^{12} \lambda_3^3 - 17 \lambda_1^{12} \lambda_3^6 - 1870 \lambda_1^9 \lambda_2^3 \lambda_3^6 - 7854 \lambda_1^6 \lambda_2^6 \lambda_3^6 - 1870 \lambda_1^3 \lambda_2^9 \lambda_3^6 - 17 \lambda_2^{12} \lambda_3^6 + 1870 \lambda_1^6 \lambda_2^3 \lambda_3^9 + 1870 \lambda_1^3 \lambda_2^6 \lambda_3^9 - 17 \lambda_1^6 \lambda_3^{12} - 170 \lambda_1^3 \lambda_2^3 \lambda_3^{12} - 17 \lambda_2^6 \lambda_3^{12} + \lambda_3^{18} + 170 \lambda_1^{12} \lambda_2^3 \lambda_4^3 - 1870 \lambda_1^9 \lambda_2^6 \lambda_4^3 + 1870 \lambda_1^6 \lambda_2^9 \lambda_4^3 - 170 \lambda_1^3 \lambda_2^{12} \lambda_4^3 + 170 \lambda_1^{12} \lambda_3^3 \lambda_4^3 - 170 \lambda_2^{12} \lambda_3^3 \lambda_4^3 + 1870 \lambda_1^9 \lambda_2^3 \lambda_4^3 - 1870 \lambda_1^6 \lambda_2^6 \lambda_4^3 + 1870 \lambda_1^3 \lambda_2^9 \lambda_4^3 - 1870 \lambda_2^6 \lambda_3^9 \lambda_4^3 + 170 \lambda_1^3 \lambda_2^{12} \lambda_4^3 - 170 \lambda_2^3 \lambda_3^{12} \lambda_4^3 - 17 \lambda_1^{12} \lambda_4^6 + 1870 \lambda_1^9 \lambda_2^3 \lambda_4^6 - 7854 \lambda_1^6 \lambda_2^6 \lambda_4^6 + 1870 \lambda_1^3 \lambda_2^9 \lambda_4^6 - 17 \lambda_2^{12} \lambda_4^6 - 1870 \lambda_1^9 \lambda_3^3 \lambda_4^6 - 1870 \lambda_2^9 \lambda_3^6 \lambda_4^6 - 7854 \lambda_1^6 \lambda_3^6 \lambda_4^6 - 7854 \lambda_2^6 \lambda_3^6 \lambda_4^6 - 1870 \lambda_1^3 \lambda_3^9 \lambda_4^6 - 1870 \lambda_2^3 \lambda_3^9 \lambda_4^6 - 17 \lambda_3^{12} \lambda_4^6 + 1870 \lambda_1^6 \lambda_2^3 \lambda_4^9 - 1870 \lambda_1^3 \lambda_2^6 \lambda_4^9 + 1870 \lambda_1^6 \lambda_3^3 \lambda_4^9 - 1870 \lambda_2^6 \lambda_3^3 \lambda_4^9 + 1870 \lambda_1^3 \lambda_3^6 \lambda_4^9 - 1870 \lambda_2^3 \lambda_3^6 \lambda_4^9 - 17 \lambda_1^6 \lambda_4^{12} + 170 \lambda_1^3 \lambda_2^{12} \lambda_4^9 - 17 \lambda_2^6 \lambda_4^{12} - 170 \lambda_1^3 \lambda_3^3 \lambda_4^{12} - 170 \lambda_2^3 \lambda_3^3 \lambda_4^{12} - 17 \lambda_3^6 \lambda_4^{12} + \lambda_4^{18}) (-117936)$$

$$f_{24} = (111 \lambda_1^{24} + 506 \lambda_1^{18} \lambda_2^6 + 10166 \lambda_1^{12} \lambda_2^{12} + 506 \lambda_1^6 \lambda_2^{18} + 111 \lambda_2^{24} - 5060 \lambda_1^{18} \lambda_2^3 \lambda_3^3 - 206448 \lambda_1^{15} \lambda_2^6 \lambda_3^3 - 1118260 \lambda_1^{12} \lambda_2^9 \lambda_3^3 - 1118260 \lambda_1^9 \lambda_2^{12} \lambda_3^3 - 206448 \lambda_1^6 \lambda_2^{15} \lambda_3^3 - 5060 \lambda_1^3 \lambda_2^{18} \lambda_3^3 + 506 \lambda_1^{18} \lambda_3^6 + 206448 \lambda_1^{15} \lambda_2^3 \lambda_3^6 + 4696692 \lambda_1^{12} \lambda_2^6 \lambda_3^6 + 12300860 \lambda_1^9 \lambda_2^9 \lambda_3^6 + 4696692 \lambda_1^6 \lambda_2^{12} \lambda_3^6 + 206448 \lambda_1^3 \lambda_2^{15} \lambda_3^6 + 506 \lambda_2^{18} \lambda_3^6 - 1118260 \lambda_1^{12} \lambda_2^3 \lambda_3^9 - 12300860 \lambda_1^9 \lambda_2^6 \lambda_3^9 - 12300860 \lambda_1^6 \lambda_2^9 \lambda_3^9 - 1118260 \lambda_1^3 \lambda_2^{12} \lambda_3^9 + 10166 \lambda_1^{12} \lambda_3^{12} + 1118260 \lambda_1^9 \lambda_2^3 \lambda_3^{12} + 4696692 \lambda_1^6 \lambda_2^6 \lambda_3^{12} + 1118260 \lambda_1^3 \lambda_2^9 \lambda_3^{12} + 10166 \lambda_2^{12} \lambda_3^{12} - 206448 \lambda_1^6 \lambda_2^3 \lambda_3^{15} - 206448 \lambda_1^3 \lambda_2^6 \lambda_3^{15} + 506 \lambda_1^6 \lambda_3^{18} + 5060 \lambda_1^3 \lambda_2^{18} \lambda_3^6 + 111 \lambda_3^{24} - 5060 \lambda_1^{18} \lambda_2^3 \lambda_4^3 + 206448 \lambda_1^{15} \lambda_2^6 \lambda_4^3 - 1118260 \lambda_1^{12} \lambda_2^9 \lambda_4^3 + 1118260 \lambda_1^9 \lambda_2^{12} \lambda_4^3 - 206448 \lambda_1^6 \lambda_2^{15} \lambda_4^3 + 506 \lambda_1^3 \lambda_2^{18} \lambda_4^3 + 5060 \lambda_1^{18} \lambda_3^6 \lambda_4^3 - 206448 \lambda_1^{15} \lambda_2^3 \lambda_4^3 + 1118260 \lambda_1^{12} \lambda_2^6 \lambda_4^3 + 1118260 \lambda_1^9 \lambda_2^9 \lambda_4^3 - 1118260 \lambda_1^6 \lambda_2^{12} \lambda_4^3 + 1118260 \lambda_1^3 \lambda_2^{15} \lambda_4^3 - 206448 \lambda_1^6 \lambda_3^{15} \lambda_4^3 + 206448 \lambda_2^6 \lambda_3^{15} \lambda_4^3 - 5060 \lambda_1^3 \lambda_3^{18} \lambda_4^3 + 5060 \lambda_2^3 \lambda_3^{18} \lambda_4^3 + 506 \lambda_1^{18} \lambda_4^6 - 206448 \lambda_1^{15} \lambda_2^3 \lambda_4^6 + 4696692 \lambda_1^{12} \lambda_2^6 \lambda_4^6 - 12300860 \lambda_1^9 \lambda_2^9 \lambda_4^6 + 4696692 \lambda_1^6 \lambda_2^{12} \lambda_4^6 - 206448 \lambda_1^3 \lambda_2^{15} \lambda_4^6 + 506 \lambda_2^{18} \lambda_4^6 + 206448 \lambda_1^{15} \lambda_3^3 \lambda_4^6 + 206448 \lambda_2^{15} \lambda_3^3 \lambda_4^6 + 4696692 \lambda_1^{12} \lambda_3^6 \lambda_4^6 + 4696692 \lambda_2^{12} \lambda_3^6 \lambda_4^6 + 12300860 \lambda_1^9 \lambda_3^9 \lambda_4^6 + 12300860 \lambda_2^9 \lambda_3^9 \lambda_4^6 +$$

$$\begin{aligned}
& 4696692 \lambda_1^6 \lambda_3^{12} \lambda_4^6 + 4696692 \lambda_2^6 \lambda_3^{12} \lambda_4^6 + 206448 \lambda_1^3 \lambda_3^{15} \lambda_4^6 + 206448 \lambda_2^3 \lambda_3^{15} \lambda_4^6 + 506 \lambda_3^{18} \lambda_4^6 - 1118260 \lambda_1^{12} \lambda_2^3 \lambda_4^9 + \\
& 12300860 \lambda_1^9 \lambda_2^6 \lambda_4^9 - 12300860 \lambda_1^6 \lambda_2^9 \lambda_4^9 + 1118260 \lambda_1^3 \lambda_2^{12} \lambda_4^9 - 1118260 \lambda_1^{12} \lambda_3^3 \lambda_4^9 + 1118260 \lambda_2^{12} \lambda_3^3 \lambda_4^9 - \\
& 12300860 \lambda_1^9 \lambda_3^6 \lambda_4^9 + 12300860 \lambda_2^9 \lambda_3^6 \lambda_4^9 - 12300860 \lambda_1^6 \lambda_3^9 \lambda_4^9 + 12300860 \lambda_2^6 \lambda_3^9 \lambda_4^9 - 1118260 \lambda_1^3 \lambda_3^{12} \lambda_4^9 + \\
& 1118260 \lambda_2^3 \lambda_3^{12} \lambda_4^9 + 10166 \lambda_1^{12} \lambda_4^{12} - 1118260 \lambda_1^9 \lambda_2^3 \lambda_4^{12} + 4696692 \lambda_1^6 \lambda_2^6 \lambda_4^{12} - 1118260 \lambda_1^3 \lambda_2^9 \lambda_4^{12} + \\
& 10166 \lambda_2^{12} \lambda_4^{12} + 1118260 \lambda_1^9 \lambda_3^3 \lambda_4^{12} + 1118260 \lambda_2^9 \lambda_3^3 \lambda_4^{12} + 4696692 \lambda_1^6 \lambda_3^6 \lambda_4^{12} + 4696692 \lambda_2^6 \lambda_3^6 \lambda_4^{12} + \\
& 1118260 \lambda_1^3 \lambda_3^9 \lambda_4^{12} + 1118260 \lambda_2^3 \lambda_3^9 \lambda_4^{12} + 10166 \lambda_1^{12} \lambda_4^{12} - 206448 \lambda_1^6 \lambda_2^3 \lambda_4^{15} + 206448 \lambda_1^3 \lambda_2^6 \lambda_4^{15} - 206448 \lambda_1^6 \lambda_3^3 \lambda_4^{15} + \\
& 206448 \lambda_2^6 \lambda_3^3 \lambda_4^{15} - 206448 \lambda_1^3 \lambda_3^6 \lambda_4^{15} + 206448 \lambda_2^3 \lambda_3^6 \lambda_4^{15} + 506 \lambda_1^6 \lambda_4^{18} - 5060 \lambda_1^3 \lambda_2^3 \lambda_4^{18} + 506 \lambda_2^6 \lambda_4^{18} + \\
& 5060 \lambda_1^3 \lambda_3^3 \lambda_4^{18} + 5060 \lambda_2^3 \lambda_3^3 \lambda_4^{18} + 506 \lambda_3^6 \lambda_4^{18} + 111 \lambda_4^{24} (28728)
\end{aligned}$$

$$\begin{aligned}
f_{30} = & (584 \lambda_1^{30} - 435 \lambda_1^{24} \lambda_2^6 - 63365 \lambda_1^{18} \lambda_2^{12} - 63365 \lambda_1^{12} \lambda_2^{18} - 435 \lambda_1^6 \lambda_2^{24} + 584 \lambda_2^{30} + 4350 \lambda_1^{24} \lambda_2^3 \lambda_3^3 + \\
& 440220 \lambda_1^{21} \lambda_2^6 \lambda_3^3 + 6970150 \lambda_1^{18} \lambda_2^9 \lambda_3^3 + 25852920 \lambda_1^{15} \lambda_2^{12} \lambda_3^3 + 25852920 \lambda_1^{12} \lambda_2^{15} \lambda_3^3 + 6970150 \lambda_1^9 \lambda_2^{18} \lambda_3^3 + \\
& 440220 \lambda_1^6 \lambda_2^{21} \lambda_3^3 + 4350 \lambda_1^3 \lambda_2^{24} \lambda_3^3 - 435 \lambda_1^{24} \lambda_3^6 - 440220 \lambda_1^{21} \lambda_2^3 \lambda_3^6 - 29274630 \lambda_1^{18} \lambda_2^6 \lambda_3^6 - 284382120 \lambda_1^{15} \lambda_2^9 \lambda_3^6 - \\
& 588153930 \lambda_1^{12} \lambda_2^{12} \lambda_3^6 - 284382120 \lambda_1^9 \lambda_2^{15} \lambda_3^6 - 29274630 \lambda_1^6 \lambda_2^{18} \lambda_3^6 - 440220 \lambda_1^3 \lambda_2^{21} \lambda_3^6 - 435 \lambda_2^{24} \lambda_3^6 + \\
& 6970150 \lambda_1^{18} \lambda_2^3 \lambda_3^9 + 284382120 \lambda_1^{15} \lambda_2^6 \lambda_3^9 + 1540403150 \lambda_1^{12} \lambda_2^9 \lambda_3^9 + 1540403150 \lambda_1^9 \lambda_2^{12} \lambda_3^9 + 284382120 \lambda_1^6 \lambda_2^{15} \lambda_3^9 + \\
& 6970150 \lambda_1^3 \lambda_2^{18} \lambda_3^9 - 63365 \lambda_1^{18} \lambda_3^{12} - 25852920 \lambda_1^{15} \lambda_2^3 \lambda_3^{12} - 588153930 \lambda_1^{12} \lambda_2^6 \lambda_3^{12} - 1540403150 \lambda_1^9 \lambda_2^9 \lambda_3^{12} - \\
& 588153930 \lambda_1^6 \lambda_2^{12} \lambda_3^{12} - 25852920 \lambda_1^3 \lambda_2^{15} \lambda_3^{12} - 63365 \lambda_2^{18} \lambda_3^{12} + 25852920 \lambda_1^{12} \lambda_3^3 \lambda_4^{15} + 284382120 \lambda_1^9 \lambda_2^6 \lambda_3^{15} + \\
& 284382120 \lambda_1^6 \lambda_2^9 \lambda_3^{15} + 25852920 \lambda_1^3 \lambda_2^{12} \lambda_3^{15} - 63365 \lambda_1^{12} \lambda_3^{18} - 6970150 \lambda_1^9 \lambda_2^3 \lambda_3^{18} - 29274630 \lambda_1^6 \lambda_2^6 \lambda_3^{18} - \\
& 6970150 \lambda_1^3 \lambda_2^9 \lambda_3^{18} - 63365 \lambda_2^{12} \lambda_3^{18} + 440220 \lambda_1^6 \lambda_2^3 \lambda_3^{21} + 440220 \lambda_1^3 \lambda_2^6 \lambda_3^{21} - 435 \lambda_1^6 \lambda_3^{24} - 4350 \lambda_1^3 \lambda_2^3 \lambda_3^{24} - \\
& 435 \lambda_2^6 \lambda_3^{24} + 584 \lambda_3^{30} + 4350 \lambda_1^{24} \lambda_2^3 \lambda_3^3 - 440220 \lambda_1^{21} \lambda_2^6 \lambda_3^3 + 6970150 \lambda_1^{18} \lambda_2^9 \lambda_3^3 - 25852920 \lambda_1^{15} \lambda_2^{12} \lambda_3^3 + \\
& 25852920 \lambda_1^{12} \lambda_2^{15} \lambda_3^3 - 6970150 \lambda_1^9 \lambda_2^{18} \lambda_3^3 + 440220 \lambda_1^6 \lambda_2^{21} \lambda_3^3 - 4350 \lambda_1^3 \lambda_2^{24} \lambda_3^3 + 4350 \lambda_1^{24} \lambda_3^3 \lambda_4^3 - 4350 \lambda_2^{24} \lambda_3^3 \lambda_4^3 + \\
& 440220 \lambda_1^{21} \lambda_3^6 \lambda_4^3 - 440220 \lambda_2^{21} \lambda_3^6 \lambda_4^3 + 6970150 \lambda_1^{18} \lambda_3^9 \lambda_4^3 - 6970150 \lambda_2^{18} \lambda_3^9 \lambda_4^3 + 25852920 \lambda_1^{15} \lambda_3^{12} \lambda_4^3 - \\
& 25852920 \lambda_2^{15} \lambda_3^{12} \lambda_4^3 + 25852920 \lambda_1^{12} \lambda_3^{15} \lambda_4^3 - 25852920 \lambda_2^{12} \lambda_3^{15} \lambda_4^3 + 6970150 \lambda_1^9 \lambda_3^{18} \lambda_4^3 - 6970150 \lambda_2^9 \lambda_3^{18} \lambda_4^3 + \\
& 440220 \lambda_1^6 \lambda_3^{21} \lambda_4^3 - 440220 \lambda_2^6 \lambda_3^{21} \lambda_4^3 + 4350 \lambda_1^3 \lambda_3^{24} \lambda_4^3 - 4350 \lambda_2^3 \lambda_3^{24} \lambda_4^3 - 435 \lambda_1^{24} \lambda_4^6 + 440220 \lambda_1^{21} \lambda_2^3 \lambda_4^6 - \\
& 29274630 \lambda_1^{18} \lambda_2^6 \lambda_4^6 + 284382120 \lambda_1^{15} \lambda_2^9 \lambda_4^6 - 588153930 \lambda_1^{12} \lambda_2^{12} \lambda_4^6 + 284382120 \lambda_1^9 \lambda_2^{15} \lambda_4^6 - 29274630 \lambda_1^6 \lambda_2^{18} \lambda_4^6 + \\
& 440220 \lambda_1^3 \lambda_2^{21} \lambda_4^6 - 435 \lambda_2^{24} \lambda_4^6 - 440220 \lambda_1^{21} \lambda_3^3 \lambda_4^6 - 440220 \lambda_2^{21} \lambda_3^3 \lambda_4^6 - 29274630 \lambda_1^{18} \lambda_3^6 \lambda_4^6 - 29274630 \lambda_2^{18} \lambda_3^6 \lambda_4^6 - \\
& 284382120 \lambda_1^{15} \lambda_3^9 \lambda_4^6 - 284382120 \lambda_2^{15} \lambda_3^9 \lambda_4^6 - 588153930 \lambda_1^{12} \lambda_3^{12} \lambda_4^6 - 588153930 \lambda_2^{12} \lambda_3^{12} \lambda_4^6 - 284382120 \lambda_1^9 \lambda_3^{15} \lambda_4^6 - \\
& 284382120 \lambda_2^9 \lambda_3^{15} \lambda_4^6 - 29274630 \lambda_1^6 \lambda_3^{18} \lambda_4^6 - 29274630 \lambda_2^6 \lambda_3^{18} \lambda_4^6 - 440220 \lambda_1^3 \lambda_3^{21} \lambda_4^6 - 440220 \lambda_2^3 \lambda_3^{21} \lambda_4^6 - \\
& 435 \lambda_3^{24} \lambda_4^6 + 6970150 \lambda_1^{18} \lambda_2^3 \lambda_4^9 - 284382120 \lambda_1^{15} \lambda_2^6 \lambda_4^9 + 1540403150 \lambda_1^{12} \lambda_2^9 \lambda_4^9 - 1540403150 \lambda_1^9 \lambda_2^{12} \lambda_4^9 + \\
& 284382120 \lambda_1^6 \lambda_2^{15} \lambda_4^9 - 6970150 \lambda_1^3 \lambda_2^{18} \lambda_4^9 + 6970150 \lambda_1^{18} \lambda_3^3 \lambda_4^9 - 6970150 \lambda_2^{18} \lambda_3^3 \lambda_4^9 + 284382120 \lambda_1^{15} \lambda_3^6 \lambda_4^9 - \\
& 284382120 \lambda_2^{15} \lambda_3^6 \lambda_4^9 + 1540403150 \lambda_1^{12} \lambda_3^9 \lambda_4^9 - 1540403150 \lambda_2^{12} \lambda_3^9 \lambda_4^9 + 1540403150 \lambda_1^9 \lambda_3^{12} \lambda_4^9 - 1540403150 \lambda_2^9 \lambda_3^{12} \lambda_4^9 + \\
& 284382120 \lambda_1^6 \lambda_3^{15} \lambda_4^9 - 284382120 \lambda_2^6 \lambda_3^{15} \lambda_4^9 + 6970150 \lambda_1^3 \lambda_3^{18} \lambda_4^9 - 6970150 \lambda_2^3 \lambda_3^{18} \lambda_4^9 - 63365 \lambda_1^{18} \lambda_4^{12} + \\
& 25852920 \lambda_1^{15} \lambda_2^3 \lambda_4^{12} - 588153930 \lambda_1^{12} \lambda_2^6 \lambda_4^{12} + 1540403150 \lambda_1^9 \lambda_2^9 \lambda_4^{12} - 588153930 \lambda_1^6 \lambda_2^{12} \lambda_4^{12} + 25852920 \lambda_1^3 \lambda_2^{15} \lambda_4^{12} - \\
& 63365 \lambda_2^{18} \lambda_4^{12} - 25852920 \lambda_1^{15} \lambda_3^3 \lambda_4^{12} - 25852920 \lambda_2^{15} \lambda_3^3 \lambda_4^{12} - 588153930 \lambda_1^{12} \lambda_3^6 \lambda_4^{12} - 588153930 \lambda_2^{12} \lambda_3^6 \lambda_4^{12} - \\
& 1540403150 \lambda_1^9 \lambda_3^9 \lambda_4^{12} - 1540403150 \lambda_2^9 \lambda_3^9 \lambda_4^{12} - 588153930 \lambda_1^6 \lambda_3^{12} \lambda_4^{12} - 588153930 \lambda_2^6 \lambda_3^{12} \lambda_4^{12} - 25852920 \lambda_1^3 \lambda_3^{15} \lambda_4^{12} - \\
& 25852920 \lambda_2^3 \lambda_3^{15} \lambda_4^{12} - 63365 \lambda_3^{18} \lambda_4^{12} + 25852920 \lambda_1^{12} \lambda_2^3 \lambda_4^{15} - 284382120 \lambda_1^9 \lambda_2^6 \lambda_4^{15} + 284382120 \lambda_1^6 \lambda_2^9 \lambda_4^{15} - \\
& 25852920 \lambda_1^3 \lambda_2^{12} \lambda_4^{15} + 25852920 \lambda_1^{12} \lambda_3^3 \lambda_4^{15} - 25852920 \lambda_2^{12} \lambda_3^3 \lambda_4^{15} + 284382120 \lambda_1^9 \lambda_3^6 \lambda_4^{15} - 284382120 \lambda_2^9 \lambda_3^6 \lambda_4^{15} + \\
& 284382120 \lambda_1^6 \lambda_3^9 \lambda_4^{15} - 284382120 \lambda_2^6 \lambda_3^9 \lambda_4^{15} + 25852920 \lambda_1^3 \lambda_3^{12} \lambda_4^{15} - 25852920 \lambda_2^3 \lambda_3^{12} \lambda_4^{15} - 63365 \lambda_1^{12} \lambda_4^{18} + \\
& 6970150 \lambda_1^9 \lambda_2^3 \lambda_4^{18} - 29274630 \lambda_1^6 \lambda_2^6 \lambda_4^{18} + 6970150 \lambda_1^3 \lambda_2^9 \lambda_4^{18} - 63365 \lambda_2^{12} \lambda_4^{18} - 6970150 \lambda_1^9 \lambda_3^3 \lambda_4^{18} - \\
& 6970150 \lambda_2^9 \lambda_3^3 \lambda_4^{18} - 29274630 \lambda_1^6 \lambda_3^6 \lambda_4^{18} - 29274630 \lambda_2^6 \lambda_3^6 \lambda_4^{18} - 6970150 \lambda_1^3 \lambda_3^9 \lambda_4^{18} - 6970150 \lambda_2^3 \lambda_3^9 \lambda_4^{18} - \\
& 63365 \lambda_3^{12} \lambda_4^{18} + 440220 \lambda_1^6 \lambda_2^3 \lambda_4^{21} - 440220 \lambda_1^3 \lambda_2^6 \lambda_4^{21} + 440220 \lambda_1^6 \lambda_3^3 \lambda_4^{21} - 440220 \lambda_2^6 \lambda_3^3 \lambda_4^{21} + 440220 \lambda_1^3 \lambda_3^6 \lambda_4^{21} - \\
& 440220 \lambda_2^3 \lambda_3^6 \lambda_4^{21} - 435 \lambda_1^6 \lambda_4^{24} + 4350 \lambda_1^3 \lambda_2^3 \lambda_4^{24} - 435 \lambda_2^6 \lambda_4^{24} - 4350 \lambda_1^3 \lambda_3^3 \lambda_4^{24} - 4350 \lambda_2^3 \lambda_3^3 \lambda_4^{24} - 435 \lambda_3^6 \lambda_4^{24} + \\
& 584 \lambda_4^{30} (-147420)
\end{aligned}$$

**0.2. Family two.** Basic semi-simple form  $p = \lambda_1 p_1 + \lambda_2 p_2 - \lambda_3 p_3$ . We randomize the  $\lambda$ 's and add the different nilpotent parts  $e$ :

Here are the corresponding adjoint rank profiles:

$$\text{N}\#3 \ e = 0: \begin{pmatrix} 0 & 0 & 78 & 78 & 0 & 0 & 0 & 78 & 0 & 234 \\ 0 & 78 & 0 & 0 & 0 & 78 & 78 & 0 & 0 & 234 \end{pmatrix}$$



$$\begin{aligned}
0.5. \quad & \textbf{Family five.} \quad e_0 e_1 e_2 + e_3 e_4 e_5 + e_2 e_3 e_6 + e_0 e_5 e_6 + e_1 e_4 e_7 + e_0 e_3 e_8 \\
& e_0 e_1 e_2 + e_3 e_4 e_5 + e_2 e_3 e_6 + e_1 e_4 e_6 + e_0 e_5 e_6 + e_1 e_3 e_7 + e_0 e_4 e_7 + e_0 e_3 e_8 \\
& e_0 e_1 e_2 + e_2 e_3 e_6 + e_0 e_5 e_6 + e_1 e_4 e_7 + e_0 e_3 e_8 \\
& e_0 e_1 e_2 + e_3 e_4 e_5 + e_0 e_3 e_6 + e_1 e_4 e_7 \\
& e_0 e_1 e_2 + e_2 e_3 e_6 + e_1 e_4 e_6 + e_0 e_5 e_6 + e_1 e_3 e_7 + e_0 e_4 e_7 + e_0 e_3 e_8 \\
& e_2 e_3 e_6 + e_0 e_5 e_6 + e_1 e_4 e_7 + e_0 e_3 e_8 \\
& e_0 e_1 e_2 + e_3 e_4 e_5 + e_1 e_3 e_6 + e_0 e_4 e_6 + e_0 e_3 e_7 \\
& e_0 e_1 e_2 + e_0 e_3 e_6 + e_1 e_4 e_7 \\
& e_2 e_3 e_6 + e_1 e_4 e_6 + e_0 e_5 e_6 + e_1 e_3 e_7 + e_0 e_4 e_7 + e_0 e_3 e_8 \\
& e_0 e_1 e_2 + e_1 e_3 e_6 + e_0 e_4 e_6 + e_0 e_3 e_7 \\
& e_0 e_3 e_6 + e_1 e_4 e_7 \\
& e_0 e_1 e_2 + e_3 e_4 e_5 + e_0 e_3 e_6 \\
& e_1 e_3 e_6 + e_0 e_4 e_6 + e_0 e_3 e_7 \\
& e_0 e_1 e_2 + e_0 e_3 e_6 \\
& e_0 e_3 e_6
\end{aligned}$$

$$e = 0: \begin{pmatrix} 0 & 0 & 70 & 70 & 0 & 0 & 0 & 70 & 0 & 210 \\ 0 & 70 & 0 & 0 & 0 & 70 & 70 & 0 & 0 & 210 \end{pmatrix}$$

$$\begin{pmatrix} 0 & 0 & 80 & 80 & 0 & 0 & 0 & 80 & 0 & 240 \\ 0 & 77 & 0 & 0 & 0 & 80 & 77 & 0 & 0 & 234 \\ 74 & 0 & 0 & 0 & 77 & 0 & 0 & 0 & 77 & 228 \\ 0 & 0 & 74 & 74 & 0 & 0 & 0 & 75 & 0 & 223 \\ 0 & 72 & 0 & 0 & 0 & 74 & 72 & 0 & 0 & 218 \\ 69 & 0 & 0 & 0 & 72 & 0 & 0 & 0 & 72 & 213 \\ 0 & 0 & 69 & 69 & 0 & 0 & 0 & 70 & 0 & 208 \\ 0 & 67 & 0 & 0 & 0 & 69 & 67 & 0 & 0 & 203 \\ 64 & 0 & 0 & 0 & 67 & 0 & 0 & 0 & 67 & 198 \\ 0 & 0 & 64 & 64 & 0 & 0 & 0 & 66 & 0 & 194 \\ 0 & 63 & 0 & 0 & 0 & 64 & 63 & 0 & 0 & 190 \\ 61 & 0 & 0 & 0 & 63 & 0 & 0 & 0 & 63 & 187 \\ 0 & 0 & 61 & 61 & 0 & 0 & 0 & 62 & 0 & 184 \\ 0 & 60 & 0 & 0 & 0 & 61 & 60 & 0 & 0 & 181 \\ 58 & 0 & 0 & 0 & 60 & 0 & 0 & 0 & 60 & 178 \\ 0 & 0 & 58 & 58 & 0 & 0 & 0 & 60 & 0 & 176 \\ 0 & 58 & 0 & 0 & 0 & 58 & 58 & 0 & 0 & 174 \\ 57 & 0 & 0 & 0 & 58 & 0 & 0 & 0 & 58 & 173 \\ 0 & 0 & 57 & 57 & 0 & 0 & 0 & 58 & 0 & 172 \\ 0 & 57 & 0 & 0 & 0 & 57 & 57 & 0 & 0 & 171 \\ 56 & 0 & 0 & 0 & 57 & 0 & 0 & 0 & 57 & 170 \\ 0 & 0 & 56 & 56 & 0 & 0 & 0 & 57 & 0 & 169 \\ 0 & 56 & 0 & 0 & 0 & 56 & 56 & 0 & 0 & 168 \end{pmatrix}$$

|    |    |    |    |    |    |    |    |     |
|----|----|----|----|----|----|----|----|-----|
| 0  | 0  | 79 | 79 | 0  | 0  | 80 | 0  | 238 |
| 0  | 76 | 0  | 0  | 0  | 78 | 76 | 0  | 230 |
| 72 | 0  | 0  | 0  | 75 | 0  | 0  | 75 | 222 |
| 0  | 0  | 71 | 71 | 0  | 0  | 73 | 0  | 215 |
| 0  | 69 | 0  | 0  | 0  | 70 | 69 | 0  | 208 |
| 66 | 0  | 0  | 0  | 68 | 0  | 0  | 68 | 202 |
| 0  | 0  | 65 | 65 | 0  | 0  | 66 | 0  | 196 |
| 0  | 63 | 0  | 0  | 0  | 65 | 63 | 0  | 191 |
| 60 | 0  | 0  | 0  | 63 | 0  | 0  | 63 | 186 |
| 0  | 0  | 60 | 60 | 0  | 0  | 62 | 0  | 182 |
| 0  | 59 | 0  | 0  | 0  | 60 | 59 | 0  | 178 |
| 58 | 0  | 0  | 0  | 59 | 0  | 0  | 59 | 176 |
| 0  | 0  | 58 | 58 | 0  | 0  | 58 | 0  | 174 |
| 0  | 57 | 0  | 0  | 0  | 58 | 57 | 0  | 172 |
| 56 | 0  | 0  | 0  | 57 | 0  | 0  | 57 | 170 |
| 0  | 0  | 56 | 56 | 0  | 0  | 57 | 0  | 169 |
| 0  | 56 | 0  | 0  | 0  | 56 | 56 | 0  | 168 |
| 0  | 0  | 78 | 78 | 0  | 0  | 78 | 0  | 234 |
| 0  | 73 | 0  | 0  | 0  | 76 | 73 | 0  | 222 |
| 68 | 0  | 0  | 0  | 71 | 0  | 0  | 71 | 210 |
| 0  | 0  | 66 | 66 | 0  | 0  | 69 | 0  | 201 |
| 0  | 64 | 0  | 0  | 0  | 64 | 64 | 0  | 192 |
| 62 | 0  | 0  | 0  | 62 | 0  | 0  | 62 | 186 |
| 0  | 0  | 60 | 60 | 0  | 0  | 60 | 0  | 180 |
| 0  | 58 | 0  | 0  | 0  | 60 | 58 | 0  | 176 |
| 56 | 0  | 0  | 0  | 58 | 0  | 0  | 58 | 172 |
| 0  | 0  | 56 | 56 | 0  | 0  | 58 | 0  | 170 |
| 0  | 56 | 0  | 0  | 0  | 56 | 56 | 0  | 168 |

|    |    |    |    |    |    |    |     |
|----|----|----|----|----|----|----|-----|
| 0  | 36 | 0  | 0  | 30 | 30 | 0  | 138 |
| 0  | 0  | 78 | 78 | 0  | 0  | 78 | 234 |
| 0  | 73 | 0  | 0  | 76 | 73 | 0  | 222 |
| 68 | 0  | 0  | 0  | 71 | 0  | 0  | 71  |
| 0  | 0  | 66 | 66 | 0  | 0  | 69 | 201 |
| 0  | 64 | 0  | 0  | 64 | 64 | 0  | 192 |
| 62 | 0  | 0  | 0  | 62 | 0  | 0  | 62  |
| 0  | 0  | 60 | 60 | 0  | 0  | 60 | 180 |
| 0  | 58 | 0  | 0  | 60 | 58 | 0  | 176 |
| 56 | 0  | 0  | 0  | 58 | 0  | 0  | 58  |
| 0  | 0  | 56 | 56 | 0  | 0  | 58 | 170 |
| 0  | 56 | 0  | 0  | 56 | 56 | 0  | 168 |

|    |    |    |    |    |    |    |    |    |     |
|----|----|----|----|----|----|----|----|----|-----|
| 0  | 0  | 78 | 78 | 0  | 56 | 0  | 0  | 56 | 56  |
| 0  | 75 | 0  | 0  | 0  | 77 | 75 | 0  | 0  | 236 |
| 70 | 0  | 0  | 0  | 74 | 0  | 0  | 0  | 74 | 218 |
| 0  | 0  | 69 | 69 | 0  | 0  | 0  | 72 | 0  | 210 |
| 0  | 67 | 0  | 0  | 0  | 68 | 67 | 0  | 0  | 202 |
| 64 | 0  | 0  | 0  | 66 | 0  | 0  | 0  | 66 | 196 |
| 0  | 0  | 63 | 63 | 0  | 0  | 0  | 64 | 0  | 190 |
| 0  | 61 | 0  | 0  | 0  | 63 | 61 | 0  | 0  | 185 |
| 58 | 0  | 0  | 0  | 61 | 0  | 0  | 0  | 61 | 180 |
| 0  | 0  | 58 | 58 | 0  | 0  | 0  | 60 | 0  | 176 |
| 0  | 57 | 0  | 0  | 0  | 58 | 57 | 0  | 0  | 172 |
| 57 | 0  | 0  | 0  | 57 | 0  | 0  | 0  | 57 | 171 |
| 0  | 0  | 57 | 57 | 0  | 0  | 0  | 56 | 0  | 170 |
| 0  | 56 | 0  | 0  | 0  | 57 | 56 | 0  | 0  | 169 |
| 56 | 0  | 0  | 0  | 56 | 0  | 0  | 0  | 56 | 168 |

|    |    |    |    |    |    |    |    |     |     |
|----|----|----|----|----|----|----|----|-----|-----|
| 0  | 0  | 77 | 77 | 30 | 0  | 0  | 78 | 0   | 232 |
| 0  | 72 | 0  | 0  | 0  | 75 | 72 | 0  | 0   | 219 |
| 68 | 0  | 0  | 0  | 70 | 0  | 0  | 70 | 208 |     |
| 0  | 0  | 66 | 66 | 0  | 0  | 0  | 67 | 0   | 199 |
| 0  | 63 | 0  | 0  | 0  | 64 | 63 | 0  | 0   | 190 |
| 60 | 0  | 0  | 0  | 61 | 0  | 0  | 0  | 61  | 182 |
| 0  | 0  | 58 | 58 | 0  | 0  | 0  | 60 | 0   | 176 |
| 0  | 57 | 0  | 0  | 0  | 58 | 57 | 0  | 0   | 172 |
| 56 | 0  | 0  | 0  | 57 | 0  | 0  | 0  | 57  | 170 |
| 0  | 0  | 56 | 56 | 0  | 0  | 0  | 57 | 0   | 169 |
| 0  | 56 | 0  | 0  | 0  | 56 | 56 | 0  | 0   | 168 |

[illegible]



2:  $e_3e_4e_5+e_2e_4e_6+e_1e_5e_6+e_1e_3e_7+e_1e_4e_7+e_0e_5e_7+e_1e_2e_8+e_0e_3e_8$

|    |    |    |    |    |    |    |    |    |     |
|----|----|----|----|----|----|----|----|----|-----|
| 0  | 0  | 79 | 79 | 0  | 0  | 0  | 80 | 0  | 238 |
| 0  | 75 | 0  | 0  | 0  | 78 | 75 | 0  | 0  | 228 |
| 70 | 0  | 0  | 0  | 74 | 0  | 0  | 0  | 74 | 218 |
| 0  | 0  | 69 | 69 | 0  | 0  | 0  | 71 | 0  | 209 |
| 0  | 66 | 0  | 0  | 0  | 68 | 66 | 0  | 0  | 200 |
| 61 | 0  | 0  | 0  | 65 | 0  | 0  | 0  | 65 | 191 |
| 0  | 0  | 60 | 60 | 0  | 0  | 0  | 62 | 0  | 182 |
| 0  | 57 | 0  | 0  | 0  | 59 | 57 | 0  | 0  | 173 |
| 52 | 0  | 0  | 0  | 56 | 0  | 0  | 0  | 56 | 164 |
| 0  | 0  | 51 | 51 | 0  | 0  | 0  | 53 | 0  | 155 |
| 0  | 48 | 0  | 0  | 0  | 50 | 48 | 0  | 0  | 146 |
| 44 | 0  | 0  | 0  | 47 | 0  | 0  | 0  | 47 | 138 |
| 0  | 0  | 43 | 43 | 0  | 0  | 0  | 44 | 0  | 130 |
| 0  | 40 | 0  | 0  | 0  | 42 | 40 | 0  | 0  | 122 |
| 36 | 0  | 0  | 0  | 39 | 0  | 0  | 0  | 39 | 114 |
| 0  | 0  | 35 | 35 | 0  | 0  | 0  | 37 | 0  | 107 |
| 0  | 33 | 0  | 0  | 0  | 34 | 33 | 0  | 0  | 100 |
| 29 | 0  | 0  | 0  | 32 | 0  | 0  | 0  | 32 | 93  |
| 0  | 0  | 28 | 28 | 0  | 0  | 0  | 30 | 0  | 86  |
| 0  | 26 | 0  | 0  | 0  | 28 | 26 | 0  | 0  | 80  |
| 22 | 0  | 0  | 0  | 26 | 0  | 0  | 0  | 26 | 74  |
| 0  | 0  | 22 | 22 | 0  | 0  | 0  | 24 | 0  | 68  |
| 0  | 20 | 0  | 0  | 0  | 22 | 20 | 0  | 0  | 62  |
| 17 | 0  | 0  | 0  | 20 | 0  | 0  | 0  | 20 | 57  |
| 0  | 0  | 17 | 17 | 0  | 0  | 0  | 18 | 0  | 52  |
| 0  | 15 | 0  | 0  | 0  | 17 | 15 | 0  | 0  | 47  |
| 12 | 0  | 0  | 0  | 15 | 0  | 0  | 0  | 15 | 42  |
| 0  | 0  | 12 | 12 | 0  | 0  | 0  | 14 | 0  | 38  |
| 0  | 11 | 0  | 0  | 0  | 12 | 11 | 0  | 0  | 34  |
| 9  | 0  | 0  | 0  | 11 | 0  | 0  | 0  | 11 | 31  |
| 0  | 0  | 9  | 9  | 0  | 0  | 0  | 10 | 0  | 28  |
| 0  | 8  | 0  | 0  | 0  | 9  | 8  | 0  | 0  | 25  |
| 6  | 0  | 0  | 0  | 8  | 0  | 0  | 0  | 8  | 22  |
| 0  | 0  | 6  | 6  | 0  | 0  | 0  | 7  | 0  | 19  |
| 0  | 5  | 0  | 0  | 0  | 6  | 5  | 0  | 0  | 16  |
| 4  | 0  | 0  | 0  | 5  | 0  | 0  | 0  | 5  | 14  |
| 0  | 0  | 4  | 4  | 0  | 0  | 0  | 4  | 0  | 12  |
| 0  | 3  | 0  | 0  | 0  | 4  | 3  | 0  | 0  | 10  |
| 2  | 0  | 0  | 0  | 3  | 0  | 0  | 0  | 3  | 8   |
| 0  | 0  | 2  | 2  | 0  | 0  | 0  | 3  | 0  | 7   |
| 0  | 2  | 0  | 0  | 0  | 2  | 2  | 0  | 0  | 6   |
| 1  | 0  | 0  | 0  | 2  | 0  | 0  | 0  | 2  | 5   |
| 0  | 0  | 1  | 1  | 0  | 0  | 0  | 2  | 0  | 4   |
| 0  | 1  | 0  | 0  | 0  | 1  | 1  | 0  | 0  | 3   |
| 0  | 0  | 0  | 0  | 1  | 0  | 0  | 0  | 1  | 2   |
| 0  | 0  | 0  | 0  | 0  | 0  | 0  | 1  | 0  | 1   |
| 0  | 0  | 0  | 0  | 0  | 0  | 0  | 0  | 0  | 0   |
| 0  | 0  | 78 | 78 | 0  | 0  | 0  | 80 | 0  | 236 |
| 0  | 74 | 0  | 0  | 0  | 76 | 74 | 0  | 0  | 224 |
| 68 | 0  | 0  | 0  | 72 | 0  | 0  | 0  | 72 | 212 |
| 0  | 0  | 66 | 66 | 0  | 0  | 0  | 69 | 0  | 201 |
| 0  | 63 | 0  | 0  | 0  | 64 | 63 | 0  | 0  | 190 |
| 57 | 0  | 0  | 0  | 61 | 0  | 0  | 0  | 61 | 179 |
| 0  | 0  | 55 | 55 | 0  | 0  | 0  | 58 | 0  | 168 |
| 0  | 52 | 0  | 0  | 0  | 54 | 52 | 0  | 0  | 158 |
| 46 | 0  | 0  | 0  | 51 | 0  | 0  | 0  | 51 | 148 |
| 0  | 0  | 45 | 45 | 0  | 0  | 0  | 48 | 0  | 138 |
| 0  | 42 | 0  | 0  | 0  | 44 | 42 | 0  | 0  | 128 |
| 37 | 0  | 0  | 0  | 41 | 0  | 0  | 0  | 41 | 119 |
| 0  | 0  | 36 | 36 | 0  | 0  | 0  | 38 | 0  | 110 |
| 0  | 33 | 0  | 0  | 0  | 35 | 33 | 0  | 0  | 101 |
| 28 | 0  | 0  | 0  | 32 | 0  | 0  | 0  | 32 | 92  |
| 0  | 0  | 27 | 27 | 0  | 0  | 0  | 30 | 0  | 84  |
| 0  | 25 | 0  | 0  | 0  | 26 | 25 | 0  | 0  | 76  |
| 21 | 0  | 0  | 0  | 24 | 0  | 0  | 0  | 24 | 69  |
| 0  | 0  | 20 | 20 | 0  | 0  | 0  | 22 | 0  | 62  |
| 0  | 18 | 0  | 0  | 0  | 20 | 18 | 0  | 0  | 56  |
| 14 | 0  | 0  | 0  | 18 | 0  | 0  | 0  | 18 | 50  |
| 0  | 0  | 14 | 14 | 0  | 0  | 0  | 16 | 0  | 44  |
| 0  | 12 | 0  | 0  | 0  | 14 | 12 | 0  | 0  | 38  |
| 10 | 0  | 0  | 0  | 12 | 0  | 0  | 0  | 12 | 34  |
| 0  | 0  | 10 | 10 | 0  | 0  | 0  | 10 | 0  | 30  |
| 0  | 8  | 0  | 0  | 0  | 10 | 8  | 0  | 0  | 26  |
| 6  | 0  | 0  | 0  | 8  | 0  | 0  | 0  | 8  | 22  |
| 0  | 0  | 6  | 6  | 0  | 0  | 0  | 7  | 0  | 19  |
| 0  | 5  | 0  | 0  | 0  | 6  | 5  | 0  | 0  | 16  |
| 4  | 0  | 0  | 0  | 5  | 0  | 0  | 0  | 5  | 14  |
| 0  | 0  | 4  | 4  | 0  | 0  | 0  | 4  | 0  | 12  |
| 0  | 3  | 0  | 0  | 0  | 4  | 3  | 0  | 0  | 10  |
| 2  | 0  | 0  | 0  | 3  | 0  | 0  | 0  | 3  | 8   |
| 0  | 0  | 2  | 2  | 0  | 0  | 0  | 2  | 0  | 6   |
| 0  | 1  | 0  | 0  | 0  | 2  | 1  | 0  | 0  | 4   |
| 1  | 0  | 0  | 0  | 1  | 0  | 0  | 0  | 1  | 3   |
| 0  | 0  | 1  | 1  | 0  | 0  | 0  | 0  | 0  | 2   |
| 0  | 0  | 0  | 0  | 0  | 1  | 0  | 0  | 0  | 1   |
| 0  | 0  | 0  | 0  | 0  | 0  | 0  | 0  | 0  | 0   |

3:  $e_2e_3e_5+e_2e_4e_6+e_1e_5e_6+e_1e_3e_7+e_1e_4e_7+e_0e_5e_7+e_1e_2e_8+e_0e_3e_8$



$$5: e_3e_4e_5+e_0e_4e_6+e_1e_5e_6+e_2e_3e_7+e_1e_4e_7+e_0e_5e_7+e_0e_2e_8+e_1e_3e_8$$

$$8: e_1e_3e_5+e_1e_3e_6+e_2e_4e_6+e_2e_3e_7+e_1e_4e_7+e_0e_5e_7+e_1e_2e_8+e_0e_3e_8$$

[illegible]

$$\begin{aligned}
12: e_3e_4e_5 + e_2e_3e_6 + e_0e_5e_6 + e_1e_5e_6 + e_0e_3e_7 + e_1e_4e_7 + e_0e_2e_8 & \begin{pmatrix} 0 & 0 & 75 & 75 & 0 & 0 & 0 & 74 & 0 & 224 \\ 0 & 66 & 0 & 0 & 0 & 71 & 66 & 0 & 0 & 203 \\ 58 & 0 & 0 & 0 & 62 & 0 & 0 & 0 & 62 & 182 \\ 0 & 0 & 54 & 54 & 0 & 0 & 0 & 55 & 0 & 163 \\ 0 & 48 & 0 & 0 & 0 & 50 & 48 & 0 & 0 & 146 \\ 41 & 0 & 0 & 0 & 44 & 0 & 0 & 0 & 44 & 129 \\ 0 & 0 & 37 & 37 & 0 & 0 & 0 & 38 & 0 & 112 \\ 0 & 31 & 0 & 0 & 0 & 34 & 31 & 0 & 0 & 96 \\ 24 & 0 & 0 & 0 & 29 & 0 & 0 & 0 & 29 & 82 \\ 0 & 0 & 22 & 22 & 0 & 0 & 0 & 25 & 0 & 69 \\ 0 & 19 & 0 & 0 & 0 & 20 & 19 & 0 & 0 & 58 \\ 15 & 0 & 0 & 0 & 17 & 0 & 0 & 0 & 17 & 49 \\ 0 & 0 & 13 & 13 & 0 & 0 & 0 & 14 & 0 & 40 \\ 0 & 10 & 0 & 0 & 0 & 11 & 10 & 0 & 0 & 31 \\ 6 & 0 & 0 & 0 & 8 & 0 & 0 & 0 & 8 & 22 \\ 0 & 0 & 4 & 4 & 0 & 0 & 0 & 7 & 0 & 15 \\ 0 & 4 & 0 & 0 & 0 & 2 & 4 & 0 & 0 & 10 \\ 2 & 0 & 0 & 0 & 2 & 0 & 0 & 0 & 2 & 6 \\ 0 & 0 & 1 & 1 & 0 & 0 & 0 & 2 & 0 & 4 \\ 0 & 1 & 0 & 0 & 0 & 1 & 1 & 0 & 0 & 3 \\ 0 & 0 & 0 & 0 & 1 & 0 & 0 & 0 & 1 & 2 \\ 0 & 0 & 0 & 0 & 0 & 0 & 0 & 1 & 0 & 1 \\ 0 & 0 & 0 & 0 & 0 & 0 & 0 & 0 & 0 & 0 \\ 0 & 0 & 75 & 75 & 0 & 0 & 0 & 76 & 0 & 226 \\ 0 & 68 & 0 & 0 & 0 & 71 & 68 & 0 & 0 & 207 \\ 60 & 0 & 0 & 0 & 64 & 0 & 0 & 0 & 64 & 188 \\ 0 & 0 & 56 & 56 & 0 & 0 & 0 & 58 & 0 & 170 \\ 0 & 51 & 0 & 0 & 0 & 52 & 51 & 0 & 0 & 154 \\ 44 & 0 & 0 & 0 & 47 & 0 & 0 & 0 & 47 & 138 \\ 0 & 0 & 40 & 40 & 0 & 0 & 0 & 42 & 0 & 122 \\ 0 & 35 & 0 & 0 & 0 & 37 & 35 & 0 & 0 & 107 \\ 28 & 0 & 0 & 0 & 32 & 0 & 0 & 0 & 32 & 92 \\ 0 & 0 & 25 & 25 & 0 & 0 & 0 & 27 & 0 & 77 \\ 0 & 21 & 0 & 0 & 0 & 22 & 21 & 0 & 0 & 64 \\ 16 & 0 & 0 & 0 & 18 & 0 & 0 & 0 & 18 & 52 \\ 0 & 0 & 14 & 14 & 0 & 0 & 0 & 14 & 0 & 42 \\ 0 & 11 & 0 & 0 & 0 & 13 & 11 & 0 & 0 & 35 \\ 8 & 0 & 0 & 0 & 10 & 0 & 0 & 0 & 10 & 28 \\ 0 & 0 & 7 & 7 & 0 & 0 & 0 & 8 & 0 & 22 \\ 0 & 6 & 0 & 0 & 0 & 6 & 6 & 0 & 0 & 18 \\ 4 & 0 & 0 & 0 & 5 & 0 & 0 & 0 & 5 & 14 \\ 0 & 0 & 3 & 3 & 0 & 0 & 0 & 4 & 0 & 10 \\ 0 & 2 & 0 & 0 & 0 & 3 & 2 & 0 & 0 & 7 \\ 0 & 0 & 0 & 0 & 2 & 0 & 0 & 0 & 2 & 4 \\ 0 & 0 & 0 & 0 & 0 & 0 & 0 & 1 & 0 & 1 \\ 0 & 0 & 0 & 0 & 0 & 0 & 0 & 0 & 0 & 0 \end{pmatrix} \\
13: e_2e_4e_5 + e_2e_3e_6 + e_1e_5e_6 + e_1e_3e_7 + e_0e_4e_7 + e_1e_2e_8 + e_0e_3e_8 & \begin{pmatrix} 0 & 0 & 74 & 74 & 0 & 0 & 0 & 76 & 0 & 224 \\ 0 & 66 & 0 & 0 & 0 & 68 & 66 & 0 & 0 & 200 \\ 56 & 0 & 0 & 0 & 60 & 0 & 0 & 0 & 60 & 176 \\ 0 & 0 & 51 & 51 & 0 & 0 & 0 & 53 & 0 & 155 \\ 0 & 44 & 0 & 0 & 0 & 46 & 44 & 0 & 0 & 134 \\ 36 & 0 & 0 & 0 & 39 & 0 & 0 & 0 & 39 & 114 \\ 0 & 0 & 31 & 31 & 0 & 0 & 0 & 32 & 0 & 94 \\ 0 & 26 & 0 & 0 & 0 & 27 & 26 & 0 & 0 & 79 \\ 20 & 0 & 0 & 0 & 22 & 0 & 0 & 0 & 22 & 64 \\ 0 & 0 & 17 & 17 & 0 & 0 & 0 & 18 & 0 & 52 \\ 0 & 13 & 0 & 0 & 0 & 14 & 13 & 0 & 0 & 40 \\ 9 & 0 & 0 & 0 & 11 & 0 & 0 & 0 & 11 & 31 \\ 0 & 0 & 7 & 7 & 0 & 0 & 0 & 8 & 0 & 22 \\ 0 & 5 & 0 & 0 & 0 & 6 & 5 & 0 & 0 & 16 \\ 2 & 0 & 0 & 0 & 4 & 0 & 0 & 0 & 4 & 10 \\ 0 & 0 & 2 & 2 & 0 & 0 & 0 & 3 & 0 & 7 \\ 0 & 1 & 0 & 0 & 0 & 2 & 1 & 0 & 0 & 4 \\ 0 & 0 & 0 & 0 & 1 & 0 & 0 & 0 & 1 & 2 \\ 0 & 0 & 0 & 0 & 0 & 0 & 0 & 0 & 0 & 0 \end{pmatrix} \\
14: e_2e_4e_5 + e_2e_3e_6 + e_1e_4e_6 + e_0e_5e_6 + e_1e_3e_7 + e_0e_4e_7 + e_1e_2e_8 + e_0e_3e_8 & \begin{pmatrix} 0 & 0 & 74 & 74 & 0 & 0 & 0 & 74 & 0 & 222 \\ 0 & 64 & 0 & 0 & 0 & 69 & 64 & 0 & 0 & 197 \\ 54 & 0 & 0 & 0 & 59 & 0 & 0 & 0 & 59 & 172 \\ 0 & 0 & 49 & 49 & 0 & 0 & 0 & 53 & 0 & 151 \\ 0 & 43 & 0 & 0 & 0 & 44 & 43 & 0 & 0 & 130 \\ 35 & 0 & 0 & 0 & 38 & 0 & 0 & 0 & 38 & 111 \\ 0 & 0 & 30 & 30 & 0 & 0 & 0 & 32 & 0 & 92 \\ 0 & 24 & 0 & 0 & 0 & 28 & 24 & 0 & 0 & 76 \\ 16 & 0 & 0 & 0 & 22 & 0 & 0 & 0 & 22 & 60$$

19:  $e_1e_3e_5 + e_2e_4e_5 + e_2e_3e_6 + e_1e_4e_6 + e_1e_2e_7 + e_0e_5e_7 + e_0e_3e_8$

|     |                                                                                     |   |    |    |    |    |    |    |    |    |    |     |     |
|-----|-------------------------------------------------------------------------------------|---|----|----|----|----|----|----|----|----|----|-----|-----|
|     |                                                                                     | ( | 0  | 0  | 73 | 73 | 0  | 0  | 0  | 76 | 0  | 222 | )   |
|     |                                                                                     |   | 0  | 65 | 0  | 0  | 0  | 69 | 65 | 0  | 0  | 199 |     |
|     |                                                                                     |   | 58 | 0  | 0  | 0  | 61 | 0  | 0  | 0  | 0  | 61  | 180 |
|     |                                                                                     |   | 0  | 0  | 54 | 54 | 0  | 0  | 0  | 55 | 0  | 163 |     |
|     |                                                                                     |   | 0  | 48 | 0  | 0  | 0  | 50 | 48 | 0  | 0  | 146 |     |
|     |                                                                                     |   | 41 | 0  | 0  | 0  | 44 | 0  | 0  | 0  | 44 | 129 |     |
|     |                                                                                     |   | 0  | 0  | 37 | 37 | 0  | 0  | 0  | 38 | 0  | 112 |     |
|     |                                                                                     |   | 0  | 31 | 0  | 0  | 0  | 33 | 31 | 0  | 0  | 95  |     |
|     |                                                                                     |   | 26 | 0  | 0  | 0  | 27 | 0  | 0  | 0  | 27 | 80  |     |
|     |                                                                                     |   | 0  | 0  | 22 | 22 | 0  | 0  | 0  | 24 | 0  | 68  |     |
|     |                                                                                     |   | 0  | 19 | 0  | 0  | 0  | 20 | 19 | 0  | 0  | 58  |     |
| 20: | $e_3e_4e_5 + e_1e_3e_6 + e_0e_4e_6 + e_2e_3e_7 + e_0e_5e_7 + e_1e_2e_8 + e_0e_3e_8$ |   | 15 | 0  | 0  | 0  | 17 | 0  | 0  | 0  | 17 | 49  |     |
|     |                                                                                     |   | 0  | 0  | 13 | 13 | 0  | 0  | 0  | 14 | 0  | 40  |     |
|     |                                                                                     |   | 0  | 10 | 0  | 0  | 0  | 11 | 10 | 0  | 0  | 31  |     |
|     |                                                                                     |   | 6  | 0  | 0  | 0  | 8  | 0  | 0  | 0  | 8  | 22  |     |
|     |                                                                                     |   | 0  | 0  | 4  | 4  | 0  | 0  | 0  | 6  | 0  | 14  |     |
|     |                                                                                     |   | 0  | 2  | 0  | 0  | 0  | 4  | 2  | 0  | 0  | 8   |     |
|     |                                                                                     |   | 1  | 0  | 0  | 0  | 2  | 0  | 0  | 0  | 2  | 5   |     |
|     |                                                                                     |   | 0  | 0  | 1  | 1  | 0  | 0  | 0  | 2  | 0  | 4   |     |
|     |                                                                                     |   | 0  | 1  | 0  | 0  | 0  | 1  | 1  | 0  | 0  | 3   |     |
|     |                                                                                     |   | 0  | 0  | 0  | 0  | 1  | 0  | 0  | 0  | 1  | 2   |     |
|     |                                                                                     |   | 0  | 0  | 0  | 0  | 0  | 0  | 0  | 1  | 0  | 1   |     |
|     |                                                                                     |   | 0  | 0  | 0  | 0  | 0  | 0  | 0  | 0  | 0  | 0   |     |
|     |                                                                                     |   | 0  | 0  | 72 | 72 | 0  | 0  | 0  | 74 | 0  | 218 | )   |
|     |                                                                                     | ( | 0  | 63 | 0  | 0  | 0  | 65 | 63 | 0  | 0  | 191 |     |
|     |                                                                                     |   | 52 | 0  | 0  | 0  | 56 | 0  | 0  | 0  | 56 | 164 |     |
|     |                                                                                     |   | 0  | 0  | 45 | 45 | 0  | 0  | 0  | 48 | 0  | 138 |     |
|     |                                                                                     |   | 0  | 38 | 0  | 0  | 0  | 38 | 38 | 0  | 0  | 114 |     |
|     |                                                                                     |   | 29 | 0  | 0  | 0  | 32 | 0  | 0  | 0  | 32 | 93  |     |
|     |                                                                                     |   | 0  | 0  | 24 | 24 | 0  | 0  | 0  | 26 | 0  | 74  |     |
|     |                                                                                     |   | 0  | 18 | 0  | 0  | 0  | 20 | 18 | 0  | 0  | 56  |     |
|     |                                                                                     |   | 12 | 0  | 0  | 0  | 15 | 0  | 0  | 0  | 15 | 42  |     |
|     |                                                                                     |   | 0  | 0  | 10 | 10 | 0  | 0  | 0  | 11 | 0  | 31  |     |
|     |                                                                                     |   | 0  | 7  | 0  | 0  | 0  | 8  | 7  | 0  | 0  | 22  |     |
|     |                                                                                     |   | 4  | 0  | 0  | 0  | 5  | 0  | 0  | 0  | 5  | 14  |     |
|     |                                                                                     |   | 0  | 0  | 3  | 3  | 0  | 0  | 0  | 2  | 0  | 8   |     |
|     |                                                                                     |   | 0  | 1  | 0  | 0  | 0  | 3  | 1  | 0  | 0  | 5   |     |
|     |                                                                                     |   | 0  | 0  | 0  | 0  | 1  | 0  | 0  | 0  | 1  | 2   |     |
|     |                                                                                     |   | 0  | 0  | 0  | 0  | 0  | 0  | 0  | 0  | 0  | 0   |     |
|     |                                                                                     |   | 0  | 0  | 72 | 72 | 0  | 0  | 0  | 74 | 0  | 218 | )   |
|     |                                                                                     | ( | 0  | 62 | 0  | 0  | 0  | 65 | 62 | 0  | 0  | 189 |     |
|     |                                                                                     |   | 52 | 0  | 0  | 0  | 55 | 0  | 0  | 0  | 55 | 162 |     |
|     |                                                                                     |   | 0  | 0  | 45 | 45 | 0  | 0  | 0  | 47 | 0  | 137 |     |
|     |                                                                                     |   | 0  | 38 | 0  | 0  | 0  | 38 | 38 | 0  | 0  | 114 |     |
|     |                                                                                     |   | 30 | 0  | 0  | 0  | 32 | 0  | 0  | 0  | 32 | 94  |     |
|     |                                                                                     |   | 0  | 0  | 25 | 25 | 0  | 0  | 0  | 26 | 0  | 76  |     |
|     |                                                                                     |   | 0  | 19 | 0  | 0  | 0  | 21 | 19 | 0  |    |     |     |

$$\begin{aligned}
25: & e_3e_4e_5 + e_1e_3e_6 + e_0e_4e_6 + e_2e_3e_7 + e_0e_5e_7 + e_1e_2e_8 \\
26: & e_1e_3e_5 + e_1e_4e_5 + e_2e_4e_6 + e_0e_5e_6 + e_0e_3e_7 + e_1e_2e_8 + e_0e_4e_8 \\
27: & e_2e_3e_4 + e_2e_3e_5 + e_0e_3e_6 + e_1e_4e_6 + e_1e_3e_7 + e_0e_5e_7 + e_0e_2e_8 \\
28: & e_2e_4e_5 + e_2e_3e_6 + e_1e_4e_6 + e_0e_5e_6 + e_1e_3e_7 + e_0e_4e_7 + e_0e_1e_8 \\
29: & e_2e_4e_5 + e_3e_4e_5 + e_0e_4e_6 + e_1e_5e_6 + e_0e_2e_7 + e_1e_3e_8
\end{aligned}$$

[illegible]



$$\begin{aligned}
33: e_1e_4e_5 + e_2e_3e_6 + e_2e_4e_6 + e_0e_5e_6 + e_0e_3e_7 + e_1e_2e_8 & \left( \begin{array}{cccccccc} 0 & 0 & 70 & 70 & 0 & 0 & 0 & 70 \\ 0 & 58 & 0 & 0 & 0 & 62 & 58 & 0 \\ 46 & 0 & 0 & 0 & 50 & 0 & 0 & 50 \\ 0 & 0 & 39 & 39 & 0 & 0 & 0 & 42 \\ 0 & 33 & 0 & 0 & 0 & 32 & 33 & 0 \\ 24 & 0 & 0 & 0 & 26 & 0 & 0 & 26 \\ 0 & 0 & 19 & 19 & 0 & 0 & 20 & 0 \\ 0 & 13 & 0 & 0 & 0 & 16 & 13 & 0 \\ 6 & 0 & 0 & 0 & 10 & 0 & 0 & 10 \\ 0 & 0 & 4 & 4 & 0 & 0 & 7 & 0 \\ 0 & 3 & 0 & 0 & 0 & 2 & 3 & 0 \\ 1 & 0 & 0 & 0 & 1 & 0 & 0 & 1 \\ 0 & 0 & 1 & 1 & 0 & 0 & 0 & 0 \\ 0 & 0 & 0 & 0 & 0 & 1 & 0 & 0 \\ 0 & 0 & 0 & 0 & 0 & 0 & 0 & 0 \\ 0 & 0 & 70 & 70 & 0 & 0 & 70 & 0 \end{array} \right) \begin{array}{c} 210 \\ 178 \\ 146 \\ 120 \\ 98 \\ 76 \\ 58 \\ 42 \\ 26 \\ 15 \\ 8 \\ 3 \\ 2 \\ 1 \\ 0 \\ 210 \end{array} \\
34: e_2e_4e_5 + e_1e_3e_6 + e_0e_4e_6 + e_2e_3e_7 + e_0e_5e_7 + e_0e_1e_8 & \left( \begin{array}{cccccccc} 0 & 0 & 70 & 70 & 0 & 0 & 0 & 70 \\ 0 & 58 & 0 & 0 & 0 & 62 & 58 & 0 \\ 46 & 0 & 0 & 0 & 50 & 0 & 0 & 50 \\ 0 & 0 & 39 & 39 & 0 & 0 & 0 & 41 \\ 0 & 30 & 0 & 0 & 0 & 32 & 30 & 0 \\ 20 & 0 & 0 & 0 & 24 & 0 & 0 & 24 \\ 0 & 0 & 14 & 14 & 0 & 0 & 16 & 0 \\ 0 & 11 & 0 & 0 & 0 & 11 & 11 & 0 \\ 6 & 0 & 0 & 0 & 8 & 0 & 0 & 8 \\ 0 & 0 & 4 & 4 & 0 & 0 & 6 & 0 \\ 0 & 2 & 0 & 0 & 0 & 2 & 2 & 0 \\ 1 & 0 & 0 & 0 & 1 & 0 & 0 & 1 \\ 0 & 0 & 0 & 0 & 0 & 0 & 0 & 0 \end{array} \right) \begin{array}{c} 210 \\ 178 \\ 146 \\ 119 \\ 92 \\ 68 \\ 44 \\ 33 \\ 22 \\ 14 \\ 6 \\ 3 \\ 0 \end{array} \\
35: e_2e_3e_5 + e_1e_4e_5 + e_1e_3e_6 + e_2e_4e_6 + e_0e_5e_6 + e_1e_2e_7 + e_0e_4e_7 + e_0e_1e_8 & \left( \begin{array}{cccccccc} 0 & 0 & 69 & 69 & 0 & 0 & 0 & 70 \\ 0 & 55 & 0 & 0 & 0 & 58 & 55 & 0 \\ 40 & 0 & 0 & 0 & 44 & 0 & 0 & 44 \\ 0 & 0 & 32 & 32 & 0 & 0 & 34 & 0 \\ 0 & 22 & 0 & 0 & 0 & 24 & 22 & 0 \\ 14 & 0 & 0 & 0 & 17 & 0 & 0 & 17 \\ 0 & 0 & 9 & 9 & 0 & 0 & 10 & 0 \\ 0 & 6 & 0 & 0 & 0 & 6 & 6 & 0 \\ 2 & 0 & 0 & 0 & 3 & 0 & 0 & 3 \\ 0 & 0 & 1 & 1 & 0 & 0 & 2 & 0 \\ 0 & 0 & 0 & 0 & 0 & 0 & 0 & 0 \end{array} \right) \begin{array}{c} 208 \\ 168 \\ 128 \\ 98 \\ 68 \\ 48 \\ 28 \\ 18 \\ 8 \\ 4 \\ 0 \end{array} \\
36(1): e_0e_3e_5 + e_1e_4e_5 + e_2e_3e_6 + e_0e_4e_6 + e_1e_3e_7 + e_2e_4e_7 + e_0e_1e_8 & \left( \begin{array}{cccccccc} 0 & 0 & 69 & 69 & 0 & 0 & 0 & 68 \\ 0 & 54 & 0 & 0 & 0 & 59 & 54 & 0 \\ 40 & 0 & 0 & 0 & 44 & 0 & 0 & 44 \\ 0 & 0 & 30 & 30 & 0 & 0 & 35 & 0 \\ 0 & 24 & 0 & 0 & 0 & 20 & 24 & 0 \\ 17 & 0 & 0 & 0 & 14 & 0 & 0 & 14 \\ 0 & 0 & 10 & 10 & 0 & 0 & 8 & 0 \\ 0 & 4 & 0 & 0 & 0 & 8 & 4 & 0 \\ 0 & 0 & 0 & 0 & 4 & 0 & 0 & 4 \\ 0 & 0 & 0 & 0 & 0 & 0 & 3 & 0 \\ 0 & 0 & 0 & 0 & 0 & 0 & 0 & 0 \\ 0 & 0 & 69 & 69 & 0 & 0 & 68 & 0 \\ 0 & 54 & 0 & 0 & 0 & 59 & 54 & 0 \\ 40 & 0 & 0 & 0 & 44 & 0 & 0 & 44 \\ 0 & 0 & 30 & 30 & 0 & 0 & 35 & 0 \\ 0 & 24 & 0 & 0 & 0 & 20 & 24 & 0 \\ 17 & 0 & 0 & 0 & 14 & 0 & 0 & 14 \\ 0 & 4 & 0 & 0 & 0 & 8 & 4 & 0 \\ 0 & 0 & 0 & 0 & 4 & 0 & 0 & 4 \\ 0 & 0 & 0 & 0 & 0 & 0 & 3 & 0 \\ 0 & 0 & 0 & 0 & 0 & 0 & 0 & 0 \end{array} \right) \begin{array}{c} 206 \\ 167 \\ 128 \\ 95 \\ 68 \\ 45 \\ 28 \\ 16 \\ 8 \\ 3 \\ 0 \\ 206 \\ 167 \\ 128 \\ 95 \\ 68 \\ 45 \\ 28 \\ 16 \\ 8 \\ 3 \\ 0 \end{array} \\
36(2) e_2e_3e_5 + e_1e_4e_5 + e_0e_4e_6 + e_1e_3e_7 + e_2e_4e_7 + e_0e_1e_8 + e_1e_2e_8 & \left( \begin{array}{cccccccc} 0 & 0 & 69 & 69 & 0 & 0 & 0 & 70 \\ 0 & 57 & 0 & 0 & 0 & 60 & 57 & 0 \\ 46 & 0 & 0 & 0 & 50 & 0 & 0 & 50 \\ 0 & 0 & 39 & 39 & 0 & 0 & 0 & 42 \\ 0 & 32 & 0 & 0 & 0 & 32 & 32 & 0 \\ 24 & 0 & 0 & 0 & 26 & 0 & 0 & 26 \\ 0 & 0 & 19 & 19 & 0 & 0 & 20 & 0 \\ 0 & 13 & 0 & 0 & 0 & 15 & 13 & 0 \\ 6 & 0 & 0 & 0 & 10 & 0 & 0 & 10 \\ 0 & 0 & 4 & 4 & 0 & 0 & 6 & 0 \\ 0 & 2 & 0 & 0 & 0 & 2 & 2 & 0 \\ 1 & 0 & 0 & 0 & 1 & 0 & 0 & 1 \\ 0 & 0 & 1 & 1 & 0 & 0 & 0 & 0 \\ 0 & 0 & 0 & 0 & 0 & 1 & 0 & 0 \\ 0 & 0 & 0 & 0 & 0 & 0 & 0 & 0 \end{array} \right) \begin{array}{c} 208 \\ 174 \\ 146 \\ 120 \\ 96 \\ 76 \\ 58 \\ 41 \\ 26 \\ 14 \\ 6 \\ 3 \\ 2 \\ 1 \\ 0 \end{array} \\
37: e_2e_3e_4 + e_1e_4e_5 + e_1e_3e_6 + e_0e_4e_6 + e_0e_5e_7 + e_1e_2e_8 & \left( \begin{array}{cccccccc} 0 & 0 & 68 & 68 & 0 & 0 & 0 & 70 \\ 0 & 55 & 0 & 0 & 0 & 57 & 55 & 0 \\ 40 & 0 & 0 & 0 & 44 & 0 & 0 & 4$$

[illegible]

[illegible]

[illegible]

$$\begin{aligned}
66: e_0e_4e_5 + e_1e_3e_6 + e_1e_2e_7 + e_0e_3e_7 + e_0e_2e_8 & \begin{pmatrix} 0 & 0 & 61 & 61 & 0 & 0 & 0 & 66 & 0 & 188 \\ 0 & 45 & 0 & 0 & 0 & 47 & 45 & 0 & 0 & 137 \\ 28 & 0 & 0 & 0 & 33 & 0 & 0 & 0 & 33 & 94 \\ 0 & 0 & 19 & 19 & 0 & 0 & 0 & 21 & 0 & 59 \\ 0 & 10 & 0 & 0 & 0 & 12 & 10 & 0 & 0 & 32 \\ 4 & 0 & 0 & 0 & 5 & 0 & 0 & 0 & 5 & 14 \\ 0 & 0 & 2 & 2 & 0 & 0 & 0 & 0 & 0 & 4 \\ 0 & 0 & 0 & 0 & 0 & 1 & 0 & 0 & 0 & 1 \\ 0 & 0 & 0 & 0 & 0 & 0 & 0 & 0 & 0 & 0 \\ 0 & 0 & 61 & 61 & 0 & 0 & 0 & 56 & 0 & 178 \\ 0 & 36 & 0 & 0 & 0 & 47 & 36 & 0 & 0 & 119 \\ 16 & 0 & 0 & 0 & 26 & 0 & 0 & 0 & 26 & 68 \\ 0 & 0 & 8 & 8 & 0 & 0 & 0 & 17 & 0 & 33 \\ 0 & 7 & 0 & 0 & 0 & 0 & 7 & 0 & 0 & 14 \\ 3 & 0 & 0 & 0 & 0 & 0 & 0 & 0 & 0 & 3 \\ 0 & 0 & 0 & 0 & 0 & 0 & 0 & 0 & 0 & 0 \\ 0 & 0 & 61 & 61 & 0 & 0 & 0 & 62 & 0 & 184 \\ 0 & 46 & 0 & 0 & 0 & 49 & 46 & 0 & 0 & 141 \\ 36 & 0 & 0 & 0 & 38 & 0 & 0 & 0 & 38 & 112 \\ 0 & 0 & 28 & 28 & 0 & 0 & 0 & 29 & 0 & 85 \\ 0 & 19 & 0 & 0 & 0 & 20 & 19 & 0 & 0 & 58 \\ 9 & 0 & 0 & 0 & 11 & 0 & 0 & 0 & 11 & 31 \\ 0 & 0 & 3 & 3 & 0 & 0 & 0 & 4 & 0 & 10 \\ 0 & 1 & 0 & 0 & 0 & 1 & 1 & 0 & 0 & 3 \\ 0 & 0 & 0 & 0 & 1 & 0 & 0 & 0 & 1 & 2 \\ 0 & 0 & 0 & 0 & 0 & 0 & 0 & 1 & 0 & 1 \\ 0 & 0 & 0 & 0 & 0 & 0 & 0 & 0 & 0 & 0 \end{pmatrix} \\
67: e_0e_3e_4 + e_1e_3e_5 + e_2e_4e_6 + e_0e_5e_6 + e_1e_2e_7 & \begin{pmatrix} 0 & 0 & 60 & 60 & 0 & 0 & 0 & 62 & 0 & 182 \\ 0 & 40 & 0 & 0 & 0 & 42 & 40 & 0 & 0 & 122 \\ 22 & 0 & 0 & 0 & 25 & 0 & 0 & 0 & 25 & 72 \\ 0 & 0 & 12 & 12 & 0 & 0 & 0 & 13 & 0 & 37 \\ 0 & 5 & 0 & 0 & 0 & 6 & 5 & 0 & 0 & 16 \\ 1 & 0 & 0 & 0 & 2 & 0 & 0 & 0 & 2 & 5 \\ 0 & 0 & 0 & 0 & 0 & 0 & 0 & 0 & 0 & 0 \end{pmatrix} \\
68: e_3e_4e_5 + e_1e_2e_6 + e_0e_3e_6 + e_0e_1e_7 + e_0e_2e_8 & \begin{pmatrix} 0 & 0 & 60 & 60 & 0 & 0 & 0 & 56 & 0 & 176 \\ 0 & 35 & 0 & 0 & 0 & 43 & 35 & 0 & 0 & 113 \\ 16 & 0 & 0 & 0 & 24 & 0 & 0 & 0 & 24 & 64 \\ 0 & 0 & 8 & 8 & 0 & 0 & 0 & 15 & 0 & 31 \\ 0 & 5 & 0 & 0 & 0 & 0 & 5 & 0 & 0 & 10 \\ 2 & 0 & 0 & 0 & 0 & 0 & 0 & 0 & 0 & 2 \\ 0 & 0 & 0 & 0 & 0 & 0 & 0 & 0 & 0 & 0 \end{pmatrix} \\
69: e_2e_3e_4 + e_1e_2e_5 + e_0e_4e_5 + e_1e_3e_6 + e_0e_2e_7 + e_0e_1e_8 & \begin{pmatrix} 0 & 0 & 59 & 59 & 0 & 0 & 0 & 62 & 0 & 180 \\ 0 & 45 & 0 & 0 & 0 & 46 & 45 & 0 & 0 & 136 \\ 28 & 0 & 0 & 0 & 32 & 0 & 0 & 0 & 32 & 92 \\ 0 & 0 & 19 & 19 & 0 & 0 & 0 & 21 & 0 & 59 \\ 0 & 8 & 0 & 0 & 0 & 10 & 8 & 0 & 0 & 26 \\ 4 & 0 & 0 & 0 & 5 & 0 & 0 & 0 & 5 & 14 \\ 0 & 0 & 1 & 1 & 0 & 0 & 0 & 0 & 0 & 2 \\ 0 & 0 & 0 & 0 & 0 & 1 & 0 & 0 & 0 & 1 \\ 0 & 0 & 0 & 0 & 0 & 0 & 0 & 0 & 0 & 0 \end{pmatrix} \\
70: e_2e_3e_4 + e_0e_2e_5 + e_1e_3e_6 + e_0e_4e_7 + e_1e_4e_7 & \begin{pmatrix} 0 & 0 & 58 & 58 & 0 & 0 & 0 & 62 & 0 & 178 \\ 0 & 39 & 0 & 0 & 0 & 41 & 39 & 0 & 0 & 119 \\ 20 & 0 & 0 & 0 & 24 & 0 & 0 & 0 & 24 & 68 \\ 0 & 0 & 11 & 11 & 0 & 0 & 0 & 11 & 0 & 33 \\ 0 & 4 & 0 & 0 & 0 & 6 & 4 & 0 & 0 & 14 \\ 1 & 0 & 0 & 0 & 1 & 0 & 0 & 0 & 1 & 3 \\ 0 & 0 & 0 & 0 & 0 & 0 & 0 & 0 & 0 & 0 \\ 0 & 0 & 58 & 58 & 0 & 0 & 0 & 56 & 0 & 172 \\ 0 & 34 & 0 & 0 & 0 & 41 & 34 & 0 & 0 & 109 \\ 16 & 0 & 0 & 0 & 22 & 0 & 0 & 0 & 22 & 60 \\ 0 & 0 & 7 & 7 & 0 & 0 & 0 & 12 & 0 & 26 \\ 0 & 4 & 0 & 0 & 0 & 0 & 4 & 0 & 0 & 8 \\ 1 & 0 & 0 & 0 & 0 & 0 & 0 & 0 & 0 & 1 \\ 0 & 0 & 0 & 0 & 0 & 0 & 0 & 0 & 0 & 0 \\ 0 & 0 & 57 & 57 & 0 & 0 & 0 & 62 & 0 & 176 \\ 0 & 35 & 0 & 0 & 0 & 43 & 35 & 0 & 0 & 113 \\ 22 & 0 & 0 & 0 & 21 & 0 & 0 & 0 & 21 & 64 \\ 0 & 0 & 8 & 8 & 0 & 0 & 0 & 15 & 0 & 31 \\ 0 & 2 & 0 & 0 & 0 & 6 & 2 & 0 & 0 & 10 \\ 2 & 0 & 0 & 0 & 0 & 0 & 0 & 0 & 0 & 2 \\ 0 & 0 & 0 & 0 & 0 & 0 & 0 & 0 & 0 & 0 \end{pmatrix} \\
71: e_0e_3e_4 + e_1e_5e_6 + e_0e_2e_7 + e_1e_2e_8 & \begin{pmatrix} 0 & 0 & 58 & 58 & 0 & 0 & 0 & 60 & 0 & 176 \\ 0 & 37 & 0 &amp$$

[illegible]

$$\begin{aligned}
92: e_0e_3e_4 + e_1e_2e_5 + e_0e_1e_6 + e_0e_2e_7 & \begin{pmatrix} 0 & 0 & 48 & 48 & 0 & 0 & 0 & 50 & 0 & 146 \\ 0 & 22 & 0 & 0 & 0 & 24 & 22 & 0 & 0 & 68 \\ 6 & 0 & 0 & 0 & 8 & 0 & 0 & 0 & 8 & 22 \\ 0 & 0 & 1 & 1 & 0 & 0 & 0 & 1 & 0 & 3 \\ 0 & 0 & 0 & 0 & 0 & 0 & 0 & 0 & 0 & 0 \end{pmatrix} \\
93: e_0e_1e_4 + e_2e_3e_5 + e_0e_2e_6 + e_1e_3e_6 & \begin{pmatrix} 0 & 0 & 48 & 48 & 0 & 0 & 0 & 50 & 0 & 146 \\ 0 & 21 & 0 & 0 & 0 & 26 & 21 & 0 & 0 & 68 \\ 8 & 0 & 0 & 0 & 7 & 0 & 0 & 0 & 7 & 22 \\ 0 & 0 & 0 & 0 & 0 & 0 & 0 & 3 & 0 & 3 \\ 0 & 0 & 0 & 0 & 0 & 0 & 0 & 0 & 0 & 0 \end{pmatrix} \\
94: e_0e_2e_3 + e_1e_4e_5 + e_0e_1e_6 & \begin{pmatrix} 0 & 0 & 45 & 45 & 0 & 0 & 0 & 46 & 0 & 136 \\ 0 & 19 & 0 & 0 & 0 & 21 & 19 & 0 & 0 & 59 \\ 4 & 0 & 0 & 0 & 5 & 0 & 0 & 0 & 5 & 14 \\ 0 & 0 & 0 & 0 & 0 & 0 & 0 & 1 & 0 & 1 \\ 0 & 0 & 0 & 0 & 0 & 0 & 0 & 0 & 0 & 0 \end{pmatrix} \\
95: e_1e_2e_3 + e_0e_1e_4 + e_0e_2e_5 + e_0e_3e_6 & \begin{pmatrix} 0 & 0 & 42 & 42 & 0 & 0 & 0 & 44 & 0 & 128 \\ 0 & 14 & 0 & 0 & 0 & 16 & 14 & 0 & 0 & 44 \\ 2 & 0 & 0 & 0 & 3 & 0 & 0 & 0 & 3 & 8 \\ 0 & 0 & 0 & 0 & 0 & 0 & 0 & 0 & 0 & 0 \end{pmatrix} \\
96: e_0e_1e_2 + e_3e_4e_5 & \begin{pmatrix} 0 & 0 & 38 & 38 & 0 & 0 & 0 & 38 & 0 & 114 \\ 0 & 19 & 0 & 0 & 0 & 20 & 19 & 0 & 0 & 58 \\ 0 & 0 & 0 & 0 & 1 & 0 & 0 & 0 & 1 & 2 \\ 0 & 0 & 0 & 0 & 0 & 0 & 0 & 1 & 0 & 1 \\ 0 & 0 & 0 & 0 & 0 & 0 & 0 & 0 & 0 & 0 \end{pmatrix} \\
97: e_0e_1e_3 + e_0e_2e_4 + e_1e_2e_5 & \begin{pmatrix} 0 & 0 & 37 & 37 & 0 & 0 & 0 & 38 & 0 & 112 \\ 0 & 10 & 0 & 0 & 0 & 11 & 10 & 0 & 0 & 31 \\ 0 & 0 & 0 & 0 & 1 & 0 & 0 & 0 & 1 & 2 \\ 0 & 0 & 0 & 0 & 0 & 0 & 0 & 0 & 0 & 0 \end{pmatrix} \\
98: e_0e_1e_2 + e_0e_3e_4 + e_0e_5e_6 + e_0e_7e_8 & \begin{pmatrix} 0 & 0 & 36 & 36 & 0 & 0 & 0 & 56 & 0 & 128 \\ 0 & 8 & 0 & 0 & 0 & 28 & 8 & 0 & 0 & 44 \\ 8 & 0 & 0 & 0 & 0 & 0 & 0 & 0 & 0 & 8 \\ 0 & 0 & 0 & 0 & 0 & 0 & 0 & 0 & 0 & 0 \end{pmatrix} \\
99: e_0e_1e_2 + e_0e_3e_4 + e_0e_5e_6 & \begin{pmatrix} 0 & 0 & 35 & 35 & 0 & 0 & 0 & 42 & 0 & 112 \\ 0 & 8 & 0 & 0 & 0 & 15 & 8 & 0 & 0 & 31 \\ 2 & 0 & 0 & 0 & 0 & 0 & 0 & 0 & 0 & 2 \\ 0 & 0 & 0 & 0 & 0 & 0 & 0 & 0 & 0 & 0 \end{pmatrix} \\
100: e_0e_1e_2 + e_0e_3e_4 & \begin{pmatrix} 0 & 0 & 30 & 30 & 0 & 0 & 0 & 32 & 0 & 92 \\ 0 & 4 & 0 & 0 & 0 & 6 & 4 & 0 & 0 & 14 \\ 0 & 0 & 0 & 0 & 0 & 0 & 0 & 0 & 0 & 0 \end{pmatrix} \\
101: e_0e_1e_2 & \begin{pmatrix} 0 & 0 & 19 & 19 & 0 & 0 & 0 & 20 & 0 & 58 \\ 0 & 0 & 0 & 0 & 1 & 0 & 0 & 0 & 1 & 1 \\ 0 & 0 & 0 & 0 & 0 & 0 & 0 & 0 & 0 & 0 \end{pmatrix}
\end{aligned}$$

## REFERENCES

*Email address:* frederic.holweck@utbm.fr

LABORATOIRE INTERDISCIPLINAIRE CARNOT DE BOURGOGNE, ICB/UTBM, UMR 6303 CNRS, UNIVERSITÉ BOURGOGNE FRANCHE-COMTÉ, 90010 BELFORT CEDEX, FRANCE

DEPARTMENT OF MATHEMATICS AND STATISTICS, AUBURN UNIVERSITY, AUBURN, AL, USA

*Email address:* oeding@auburn.edu

DEPARTMENT OF MATHEMATICS AND STATISTICS, AUBURN UNIVERSITY, AUBURN, AL, USA
